# Supplementary material for: Self-propelled chimeras
Source: arXiv:1511.04738 source file (2018-10-11)
Supplement: Supplementary file 1 [file supplemental_material_rr.pdf]

# Supplemental Material for “Self-propelled Chimeras”

Nikita Kruk<sup>1</sup>, Yuri Maistrenko<sup>1,2</sup>, Nicolas Wenzel<sup>1</sup>, and Heinz Koeppl<sup>1</sup>

<sup>1</sup>*Department of Electrical Engineering and Information Technology,  
Technische Universitaet Darmstadt, Darmstadt, Germany and*

<sup>2</sup>*Institute of Mathematics and Center for Medical and Biotechnical Research,  
National Academy of Sciences of Ukraine, Kyiv, Ukraine*

(Dated: October 16, 2015)

## S.1 ALTERNATIVE SPACE-TIME PLOTS

The space-time plots for chimera states in Fig. 2 of the main text are reordered at each time step so as to guarantee that the coherent cluster is always in the center of the plots. However, in Fig. S1 global ordering of particles is applied once, with respect to the distance to the maximal density point when averaged over all the simulation time interval, with the particle of the smallest such distance placed in the center; temporal averaging of 100 time units is applied. The characteristics of chimera states can still be identified in this alternative representation and moreover the escape and capture process as discussed in the main text becomes apparent.

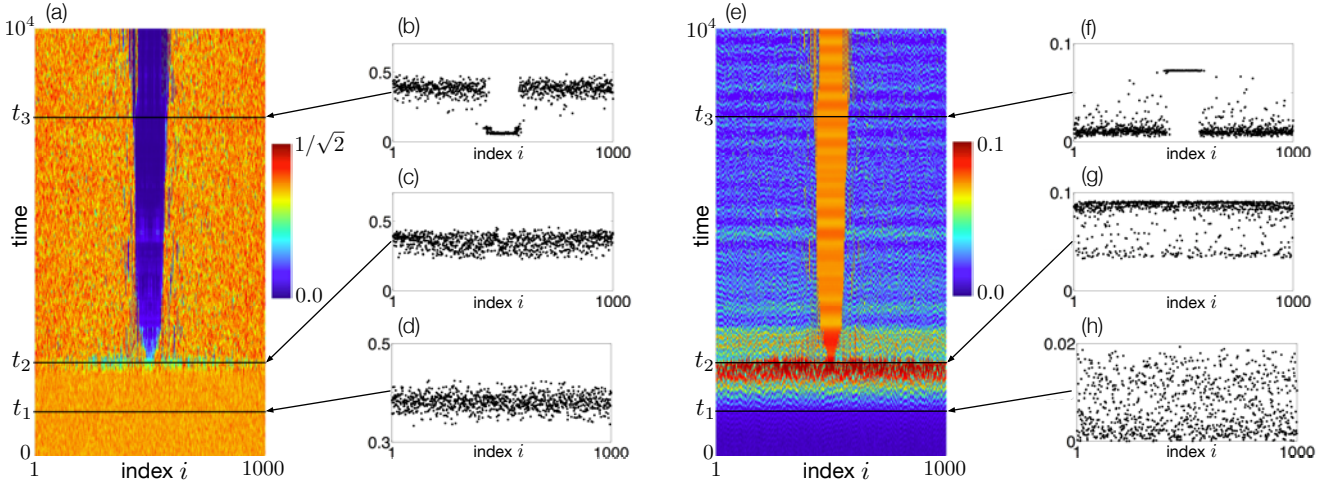

FIG. S1: (Color online) Space-time plots for a chimera state in an SPP system characterized by means of localization (a) and phase velocity (e) measures (color coding) (cf. Fig. 2); (b),(c),(d) and (f),(g),(h) instantaneous values of (a) and (e), respectively, at time units  $t_1 = 1000$ ,  $t_2 = 2100$  and  $t_3 = 8000$ , respectively; parameters:  $\sigma = 1.0$ ,  $\rho = 0.25$ ,  $\alpha = 1.53$ ,  $N = 1000$ .

## S.2 GLOBAL AND LOCAL ORDER PARAMETERS

An important characteristic of coupled oscillators is the Kuramoto order parameter which in the case of SPP systems is the averaged normalized velocity (Fig. S2(a))

$$\kappa(t) = \left\| \frac{1}{N} \sum_{i=1}^N v(\varphi_i(t)) \right\|. \quad (1)$$

However, as it is a global characteristic of the system behavior, it provides only limited insight in the dynamics of SPP systems. In the case of self-propelled chimera state, which implies simultaneous existence of two clusters: one polarized and localized in space, the other phase-incoherent and spatially distributed, the value of  $\kappa$  is intermediate, which is not reflecting the actual state of the system.

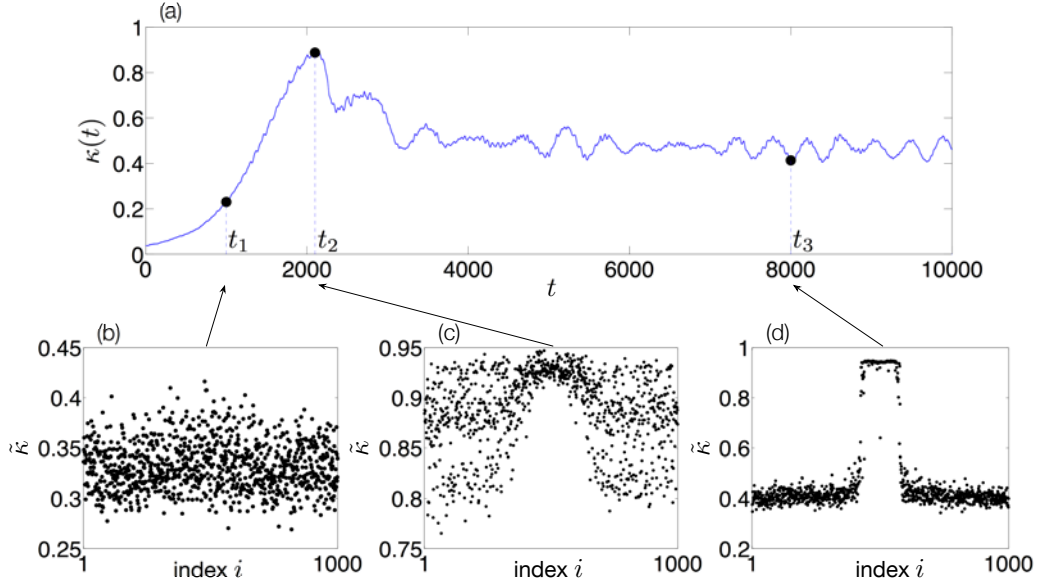

FIG. S2: (Color online) (a) Global order parameter  $\kappa(t)$  versus time  $t$ . (b),(c),(d) Local order parameter  $\tilde{\kappa}$  at time units  $t_1 = 1000$ ,  $t_2 = 2100$ , and  $t_3 = 8000$ . Ordering of particles corresponds to the distance to the maximal density point (cf. Fig. S1). Parameters:  $\sigma = 1.0$ ,  $\rho = 0.25$ ,  $\alpha = 1.53$ ,  $N = 1000$ .

The existence of the self-propelled chimera can be detected by the local version of the order parameter (Fig. S2(b-d))

$$\tilde{\kappa}_i = \left\| \frac{1}{|B_\rho^i|} \sum_{j \in B_\rho^i} v(\varphi_j(t)) \right\|, \quad (2)$$

which is equal 1 only when the particle from the neighborhood  $B_\rho^i$  are all aligned. If the value is high, the existence of the localized group is guaranteed, however, it is not guaranteed that there exists only one group. So in the case of two localized groups, the parameter  $\tilde{\kappa}$  is also not of a great use.

### S.3 CAPTION TO THE MOVIES

The movies show the dynamics of chimeras in a unit square  $[0, 1] \times [0, 1]$  with periodic boundary conditions. Numerical solutions of particle dynamics were obtained using a Runge-Kutta solver DOPRI5. Color code of each particle corresponds to its frequency (a rate of change of phase  $\dot{\varphi}$ ) with blue for the smallest and red for the highest frequency values.

*Video S1* Emergence of localized directional one-headed chimera state starting from random initial conditions. Parameters:  $\sigma = 1.0$ ,  $\rho = 0.25$ ,  $\alpha = 1.53$ ,  $N = 1000$ .

*Video S2* Emergence of localized directional two-headed chimera state starting from random initial conditions. Parameters:  $\sigma = 1.0$ ,  $\rho = 0.08$ ,  $\alpha = 1.35$ ,  $N = 1000$ .

*Video S3* Emergence of scattered directional chimera state without localization starting from random initial conditions. Parameters:  $\sigma = 1.0$ ,  $\rho = 0.05$ ,  $\alpha = 1.505$ ,  $N = 1000$ .

*Video S4* Emergence of localized directional one-headed chimera state starting from random initial conditions. Parameters:  $\sigma = 4.0$ ,  $\rho = 0.25$ ,  $\alpha = 1.53$ ,  $N = 1000$ .

*Video S5* Emergence of localized directional one-headed chimera state starting from random initial conditions. Parameters:  $\sigma = 10.0$ ,  $\rho = 0.25$ ,  $\alpha = 1.53$ ,  $N = 1000$ .

*Video S6* Emergence of localized directional one-headed chimera state starting from random initial conditions according to the extended model (see (8) in the main text) with the following alignment function

$$G(r) = \begin{cases} 1 & \text{if } r \leq \rho - \delta, \\ \frac{1}{2} - \frac{1}{2} \cos(\pi \frac{r-\rho}{\delta}) & \text{if } r < \rho \\ 0 & \text{if } r \geq \rho \end{cases}.$$

Parameters:  $\sigma = 1.0$ ,  $\rho = 0.25$ ,  $\alpha = 1.53$ ,  $\delta = 0.01$ ,  $\mu = 0$ ,  $N = 1000$ .

*Video S7* Emergence of localized directional one-headed chimera state starting from random initial conditions according to the extended model (8) with the cohesion function corresponding to the Morse-type potential

$$U(r) = C_R e^{-r/l_R} - C_A e^{-r/l_A}.$$

Parameters:  $\sigma = 1.0$ ,  $\rho = 0.2$ ,  $\alpha = 1.525$ ,  $\delta \rightarrow 0$ ,  $\mu = 0.01$ ,  $N = 1000$ ,  $C_R = 0.1$ ,  $C_A = 0.001$ ,  $l_R = 0.001$ ,  $l_A = 0.1$ .
